# Supplementary material for: Importance of electron correlations in understanding the photo-electron spectroscopy and the Weyl character of MoTe$_2$
Source: arXiv:1808.06445 source file (2018-08-20)
Supplement: Supplementary file 1 [file Supplementary_Information.pdf]

# Importance of electronic interaction in the electronic structure of type-II Weyl semimetallic candidate $\gamma-$ $MoTe_2$-Supplemental material

Niraj Aryal[(1)] and Efstratios Manousakis[(1,2)]
[(1)] *Department of Physics and National High Magnetic Field Laboratory, Florida State University, Tallahassee, FL 32306-4350, USA*
[(2)] *Department of Physics, University of Athens, Panepistimioupolis, Zografos, 157 84 Athens, Greece*
(Dated: August 7, 2018)

## I. COMPUTATIONAL DETAILS

The ab-initio calculations for $MoTe_2$ are carried out using the Quantum Espresso[1] implementation of the density functional theory (DFT) in the GGA framework including spin-orbit coupling (SOC). The Perdew-Burke-Ernzerhof (PBE) exchange correlation functional[2] was used with fully relativistic norm conserving pseudopotentials generated using the optimized norm-conserving Vanderbilt pseudopotentials as described in Ref. 3. All GGA+U calculations presented in this paper are done within the rotationally invariant scheme of Liechtenstein *et al.*[4]. We used a $k$-mesh of $15 \times 9 \times 5$ to sample the BZ for the self-consistent calculations and also an energy cutoff of 650 eV was used after carrying out careful convergence tests. The Fermi surface sheets were visualized using the XCrysden software[5]. The angular dependence of the quantum oscillation frequencies was calculated using the skeaf code[6]. Wannier90[7] software was used to construct a tight binding Hamiltonian consisting of Mo $4d$ and Te $5p$ states without maximal localization procedure. The Wannierisation method enabled us to calculate the Fermi surface, band structure and Berry curvature using a very dense k-mesh. The constructed tight binding Hamiltonian was fed into WannierTools software[8] to calculate the slab band structure, slab Fermi surface and to identify the Weyl points.

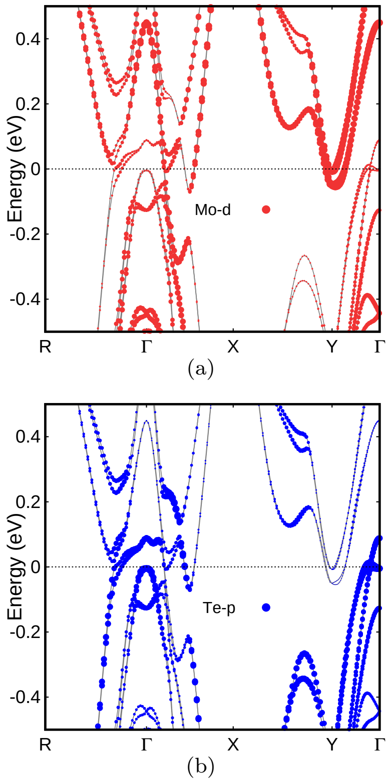


FIG. 1. Band structure of $MoTe_2$ obtained from GGA calculation along $R-\Gamma-X-Y-\Gamma$ high symmetry directions showing the projection onto (a) Mo-$d$ orbitals and (b) Te-$p$ orbitals. The size of the dots is proportional to the percentage of the corresponding orbitals. The contributions from other orbitals are negligible, hence not shown here for clarity.

## II. BAND STRUCTURE AND FERMI SURFACE

### A. Orbital projected band structure

In Figs. 1(a) and 1(b), we present the projected band structure of $MoTe_2$ onto the Mo-$d$ and Te-$p$ orbitals respectively. The contribution from other orbitals close to the Fermi level is negligible, hence we focused on only these two kind of orbitals. It is seen that the electron and hole bands have hybridization of the Mo-$d$ and Te-$p$ orbitals.

### B. Band-structure as a function of U

In Fig. 2, we present the band structure of $MoTe_2$ obtained by using different values of U.

### C. Fermi surface and its evolution

Since the biggest disagreement with the quantum oscillation (QO) experiments arises from the absence of the large-sized orbits ($\geq$ 1500T) which correspond to the hole pockets in the DFT calculations, we focus only on these hole pockets. In Fig. 3(a) we illustrate how the biggest of the hole pockets evolve as a function of U for the values of U ranging from 0 (i.e. DFT) to $5eV$. In Fig. 3(b), we show the calculated angular dependence for different values of U. The size of the hole pockets decrease as a function of U. Notice how the frequency at $c$-axis collapses from 1500 T to 500 T when varying U from 4 to

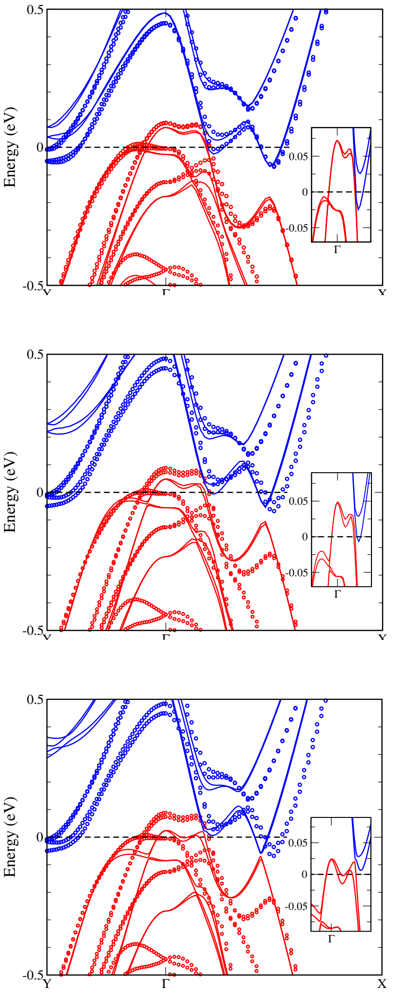


(c)

FIG. 2. Band Structure of $MoTe_2$ with the inclusion of spin-orbit-coupling (SOC) using a Hubbard U on the Mo *d*-orbital of (a) 2 eV (b) 4 eV (c) 5 eV. The dotted lines are the result of GGA (i.e. U = 0 ) in order to compare the bands before and after the application of U. The inset shows the zoomed version of the band structure for U = 2 and U = 5 eV respectively. Notice that in (c), both the hole pockets are “sunk” inside the Fermi sea close to the Γ-point.

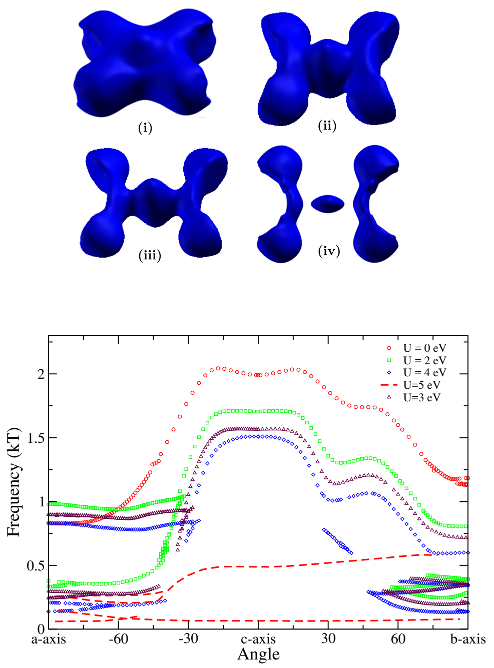


(b)

FIG. 3. (a) Evolution of the biggest hole pocket for different values of U (i) U=0 (ii) U = 2 and (iii) U = 4 eV (iv) U=5 eV. (b) Comparison of the angular dependence of the hole pocket shown in (a) for different values of U.

5 eV because of a Lifshitz transition. This is seen in Fig. 3(a) (iv) where the central part of the hole pocket separates from the “kidneys”.

### D. Comparison with experimental angular dependence

In the main text, we presented the comparison between the calculated and the angular dependence of the Fermi surface as obtained by quantum oscillation (QO) experiments by averaging the spin-orbit partners in our calculations. This is because the spin-orbit partners seen in the experiments had much less splitting than that seen in our calculations. In this section, we show the comparison without averaging the spin-orbit partners. Fig. II D shows the angular dependence of the electron and hole pockets for both of the spin-orbit partners obtained from the DFT calculation. As can be concluded by examining this Figure, because of the large size of the effect of the SOC on the orbits not seen in the QO experiments, prevents us from making any meaningful comparison. In the QO experiments there are two very close to each other frequencies for every orbit, which have been interpreted in Ref. 9 as the SO partners. When averaging both frequencies in each of these pairs in the experimental data and in the DFT calculations the identification of the orbits becomes clearer.

### E. Fate of the Weyl points

First, we identify the position of each Weyl point for our $MoTe_2$ crystal by looking at the Berry curvature vector plot for $k_z = 0$ in Fig. 5(a). Our calculation shows Weyl points at $W_1 = (0.102\frac{2\pi}{a}, 0.058\frac{2\pi}{b}, 0.0)$ and $W_2 = (0.104\frac{2\pi}{a}, 0.017\frac{2\pi}{b}, 0.0)$. The Figure clearly shows the source and the sink of the Berry curvature as marked by $W_2$ and $W_1$ respectively. In total, there are 4 pairs of Weyl points, each on one quadrant, all of which are lo-

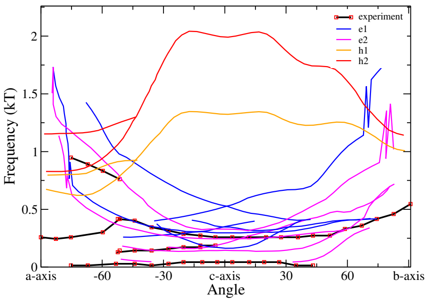


FIG. 4. Comparison between the experimental angular dependence and the calculated angular dependence for (a) DFT (b) U=3 eV (to be made) without averaging the spin-orbit partners.

cated at the $k_z = 0$ plane and are related by the crystal symmetry. The Berry curvature vector plot for $U = 0.75$ eV is shown in Fig. 5(b) which shows that the position of the Weyl point has changed.

Our calculation finds that though the number and position of Weyl points change as a function of U, some pairs of Weyl points survive the introduction of U. The band structure along one such pair of Weyl points is shown in Fig. 6 for different values of U.

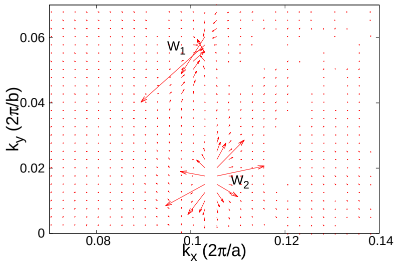


(a)

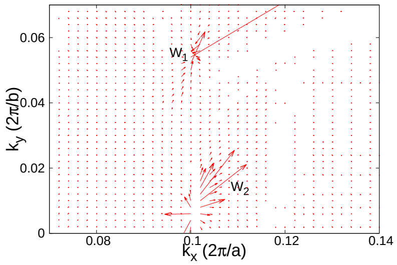


(b)

FIG. 5. Fig. (a) and Fig. (b) show the vector plot of the $x$ and $y$ component of the Berry curvature on the $k_z = 0$ plane around the Weyl points for $U = 0$ and $U = 0.75$ eV respectively. The relative size of the length of the vector is proportional to the magnitude of the Berry curvature.

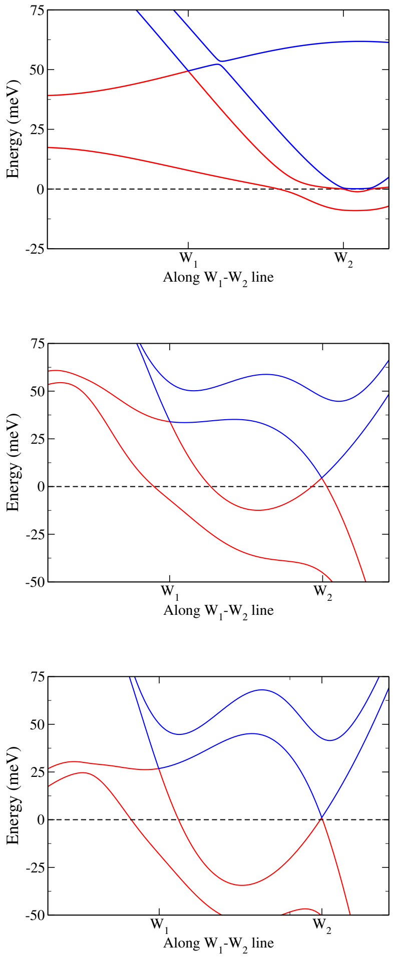


(c)

FIG. 6. Band structure along the Weyl points $W_1$ and $W_2$ for (a) $U = 2$ eV and (b) $U = 4$ eV. Notice the transition of $W_2$ Weyl point from type-II to type-I from U=0 to U=2 and beyond. Notice that the Weyl points move towards $E_F$ for non-zero U.

## III. MATRIX ELEMENTS EFFECTS IN ARPES

We start by recalling the very general expression for the ARPES intensity[10–13] in the one-step model, i.e.,

$$I = \frac{e\hbar}{mc} \sum_i B_{ii} |\vec{A} \cdot \langle f|\vec{p}|i\rangle|^2, \quad (1)$$

where $B_{ii}$ are the corresponding matrix elements of the imaginary part of the retarded single-electron Green's function $G_1^+$ (i.e., the spectral function) in the basis formed by all the initial states $|i\rangle$ of the electronic system in the solid, i.e.,

$$B_{ii} = -\frac{1}{\pi} \langle i|ImG_1^+|i\rangle. \quad (2)$$

Here the electromagnetic vector potential is a vector parallel to the direction $\vec{\epsilon}$ of the polarization of the incident photon.

Here we wish to identify for a given direction of the light polarization which orbital characters of each band does not contribute to the ARPES intensity.

We will consider the usual geometry of scattering in ARPES where the detected photo-ejected electron has momentum parallel to the surface[10], i.e.,

$$|f\rangle = |\mathbf{k}_{||}\rangle, \tag{3}$$
$$\langle \vec{r}|\mathbf{k}_{||}\rangle \sim e^{i(k_x x + k_y y)}, \tag{4}$$

where the $x$ and $y$ directions are the two directions parallel to the slab surface in our calculation. The initial state is usually expanded within the unit cell as[10]

$$\langle \vec{r}|i\rangle = \sum_{l,m,\alpha} i^l C^{\alpha}_{l,m} R^{\alpha}_l(r) Y_{l,m}(\theta,\omega), \tag{5}$$

where $\alpha$ denotes different basis states and $R^{\beta}_l(r)$ is the radial part of the Bloch wavefunction. In our case the states under consideration contributing to the ARPES intensity are mixtures of $p$ and $d$ character only. Therefore, we write

$$\langle \vec{r}|i\rangle = \sum_{l,\nu\alpha} i^l D^{\alpha}_{l,\nu} \mathcal{R}^{\alpha}_l(r) Q_{l\nu}(x,y,z), \tag{6}$$

where $Q_{l\nu}$ are the familiar linear combinations of the $Y_{l,m}$ for a given fixed value of $l$ and for $l = 1$ they are

$$Q_{11}(x,y,z) = p_x, \tag{7}$$
$$Q_{12}(x,y,z) = p_y, \tag{8}$$
$$Q_{13}(x,y,z) = p_z. \tag{9}$$

and for $l = 2$

$$Q_{21}(x,y,z) = d_{z^2}, \tag{10}$$
$$Q_{22}(x,y,z) = d_{x^2-y^2}, \tag{11}$$
$$Q_{23}(x,y,z) = d_{xy}, \tag{12}$$
$$Q_{24}(x,y,z) = d_{xz}, \tag{13}$$
$$Q_{25}(x,y,z) = d_{yz}. \tag{14}$$

Notice that because $\mathcal{R}_l(r)$ is an even function of $x$, $y$ and $z$, and because the final state given by Eq. 4 is only a function of $x$ and $y$, using the form given in Eq. 6 as initial states, it is straightforward to show that the matrix elements of the operator $\vec{\epsilon}\cdot\nabla$ which enters in Eq. 1 follows the following rules for the different orbital character of the components of each band:

(a) When $\vec{\epsilon}||\hat{z}$ from the $p$-orbitals only the $p_z$ character contributes to the intensity. From the $d$-orbitals only the $d_{xz}$ and $d_{yz}$ contribute.

(b) When $\vec{\epsilon} \perp \hat{z}$ from the $p$-orbitals only the $p_x$ and $p_y$ character contribute to the intensity. From the $d$-orbitals only the $d_{xy}$ and $d_{x^2-y^2}$ and $d_{z^2}$ contribute.

## IV. A SIMPLE MODEL OF WEYL SEMIMETAL

We present a simple $4 \times 4$ lattice model of a Weyl semimetal in order to demonstrate that the Weyl points can be destroyed or created by the action of a Hubbard term and we treat the electronic correlation term within mean-field theory. This corresponds to the GGA+U approach where the on-site Coulomb repulsion term is also factorized as in the MFT. Though our goal in this paper is to understand the effect of U in $MoTe_2$ specifically, our model is general enough to explain the role of U in the other type-II Weyl candidate, $WTe_2$, which is of the same crystal family as $MoTe_2$.

Since the bands forming Weyl points in $MoTe_2$ are comprised of hybridised Mo-$d$ and Te-$p$ orbitals, we can write an effective 4-band model using these two hybridised orbitals along with the spin degree of freedom as our basis. However, as seen in Fig. 1, they are not of pure $d$ or $p$ character; hence the effect of the Hubbard U term on the Mo $d$-orbital on each of the bands will be proportional to the product of the U value and the percentage of $d$ orbital in each of the bands. We will call these orbitals A and B, where orbital A refers to the orbital having higher proportion of Mo-$d$ (i.e. $d$-like) and B refers to the orbital having higher proportion of Te-$p$ orbital (i.e. $p$-like). Hence, our basis consists of the following four states: $|A\uparrow\rangle, |B\uparrow\rangle, |A\downarrow\rangle, |B\downarrow\rangle$.

### A. A 2D Weyl model

First, we write a continuum version of the 2D Dirac model which are centered around $(k^0_x, k^0_y)$. These Dirac points will be converted to Weyl points after the addition of spin-orbit coupling (SOC) term. In the following subsection, we will discuss a 3D model obtained from this 2D model by stacking these 2D planes on top of each other. Our Hamiltonian for the 2D-Dirac point can be written as:

$$H(\vec{k}) = \begin{bmatrix} 0 & k'^- & 0 & 0 \\ k'^+ & 0 & 0 & 0 \\ 0 & 0 & 0 & k'^- \\ 0 & 0 & k'^+ & 0 \end{bmatrix}, \tag{15}$$

where $k^{\pm} = k_x \pm ik_y$ and $k'_{x(y)} = k_{x(y)} - k^0_{x(y)}$.

With the inclusion of a Rashba type spin-orbit interaction of the form $2\lambda(\vec{\sigma}\times\vec{k}).\hat{z}$ that introduces spin-hopping from A sublattice to B and vice-versa, our Hamiltonian becomes:

$$H(\vec{k}) = \begin{bmatrix} 0 & k'^- & 0 & 2\lambda ik^- \\ k'^+ & 0 & 2\lambda ik^- & 0 \\ 0 & -2\lambda ik^+ & 0 & k'^- \\ -2\lambda ik^- & 0 & k'^+ & 0 \end{bmatrix}. \tag{16}$$

This model gives eigenvalues $E = \pm\sqrt{X}$ where, $X = |k'^2| + 4\lambda^2|k^2| \pm 4\lambda k'_x|k|$. The expression for $X$ can be rewritten as $X = k'^2_y + (k'_x \pm 2\lambda|k|)^2$. Thus, $X = 0$

when $k'_y = 0$ and $k_x = k_x^0 + 2\lambda|k|$. The condition for $k_x$ gives two values of $k_x$ where zero energy occurs, i.e., at $\kappa_x^{\pm} = k_x^0 \pm \sqrt{k_x^{0^2} - (1-4\lambda^2)(k_x^{0^2} - 4\lambda^2 k_y^{0^2})}$. $\kappa_x^{\pm}$ is real if $\frac{(1-4\lambda^2)(k_x^{0^2} - 4\lambda^2 k_y^{0^2})}{k_x^{0^2}} \leq 1$. In particular, for $k_x^0 = k_y^0$, we find that we have two zero energy solutions if $\lambda^2 \leq 0.5$. In general, the existence of Weyl points depends on the value of $\lambda, k_x^0$ and $k_y^0$. In Figs. 7(b) and 7(c), we show the dispersion for values of the Rashba coupling parameter 0 and 0.2 respectively. The former one gives a Dirac cone whereas the latter one gives two Weyl nodes separated along the $k_x$ direction.

### B. A 3D Weyl model

Having understood the effect of a Rashba term in this 2D Dirac model, we wish to address the problem which more relevant to our system of $\gamma$-$MoTe_2$. In $\gamma$-$MoTe_2$, since the $d$ and $p$ orbitals contributing to the Weyl points arise from two different atoms, it is more realistic to consider different onsite energies, say $E_A$ and $E_B$ for the two orbitals. Hence, our Hamiltonian for the 2D-Weyl point take the following form:

$$H_{2D}(\mathbf{k}) = \epsilon \hat{I} + \begin{bmatrix} \delta E & k'^{-} & 0 & 2\lambda i k^{-} \\ k'^{+} & -\delta E & 2\lambda i k^{-} & 0 \\ 0 & -2\lambda i k^{+} & \delta E & k'^{-} \\ -2\lambda i k^{-} & 0 & k'^{+} & -\delta E \end{bmatrix} \quad (17)$$

where, $\epsilon = \frac{(E_A+E_B)}{2}$, $\delta E = \frac{(E_A-E_B)}{2}$, and $\hat{I}$ is the $4\times4$ identity matrix.

Since the identity term in Eqn. 17 is just a momentum-independent overall shift of the bands, we will neglect it in the following discussion. The eigenvalues of Eqn. 17 are given by $E = \pm\sqrt{(\delta E)^2 + X}$ which yield gapped Weyl points when $E_A \neq E_B$ .

Now, we will stack these gapped 2D Weyl planes along the $z$ direction to form a quasi-2D crystal which can describe the weak interlayer coupling in these exfoliable materials. Such an approach of constructing higher dimensional topological systems from lower dimensional topological systems have been applied before in Refs. 14 and 15. In doing so, we will consider the effective hopping from A to A orbital to be different from the hopping from B to B orbital. This is realistic for materials like $MoTe_2$ and $WTe_2$ because the crystal structure, shown in Fig. 7(a), consists of buckled planes of Mo and Te atoms. In this case the out-of-plane Te-Te atomic distance is smaller than that of the Mo-Mo case. In fact, for these materials, the Mo-Mo distance is even larger than Te-Mo distance, which allows us to even neglect the hopping from Mo-Mo orbitals; however, our qualitative results remain unaffected by either of these two approaches. By using different onsite energies on A and B orbitals and/or different effective hoppings between the same orbitals, we break the inversion symmetry in our model.

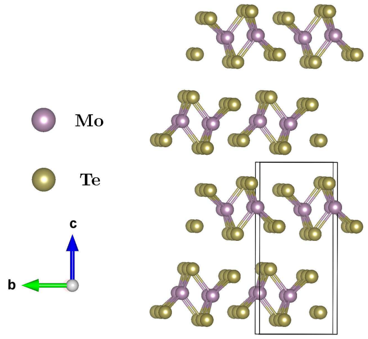


(a)

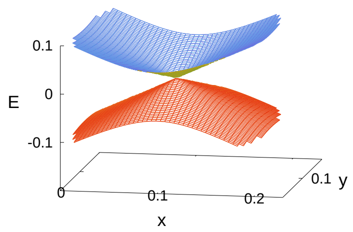


(b)

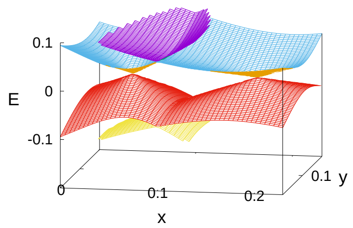


(c)

FIG. 7. (a) Crystal structure of $MoTe_2$. The black solid line gives the boundary of the unit cell. Notice the "stacking" of Mo and Te planes along the $c$ axis. (b) and (c) shows the birth of Weyl points out of the Dirac point due to the Rashba term for the 2-D model. In (b) the Dirac cone is four-fold degenerate and centered at (0.1,0.1) whereas in (c) the Dirac cone forms two Weyl points at $(0.0544, 0.1)$ and $(0.1835, 0.1)$ for a value of the Rashba coupling constant $\lambda = 0.2$.

Now the Hamiltonian for a 3D lattice becomes:

$$H_{3D}(\mathbf{k}) = -2t_{AB}\cos(k_z)\hat{I} + H'_{2D}(\mathbf{k}), \quad (18)$$

where, $H'_{2D}(\mathbf{k})$ is similar to $H_{2D}(\mathbf{k})$ except the diagonal $\delta E$ term is replaced by $Y = \delta E - 2\delta t_z \cos(k_z c)$ such that $\delta t_z = \frac{(t_A - t_B)}{2}$ and $t_{AB} = \frac{(t_A+t_B)}{2}$. The introduction of the "buckling" along the $z$-direction in our Hamiltonian gives back the Weyl physics which was gapped in the 2D case because $E = \pm\sqrt{Y^2 + X}$ and $Y = 0$ if $\delta E = -\delta t_z \cos(k_z c)$. Hence, the zero energy solution occurs for $(\kappa_x^{\pm}, k_y^0, \kappa_z)$ where, $\kappa_z c = \cos^{-1}(\frac{\delta E}{2\delta t_z}))$ and the

solution exists if $2|\delta t_z| \geq |\delta E|$. Note that the $k_z$ dependent identity term makes the Weyl cone always of type-II nature with a tilt along the $k_z$ direction because $2t_{AB} \geq |\delta t_z|$. Let us analyze the following two conditions:

1. For the equality condition, we obtain a zero energy solution for $k_z c = \pi$. This gives linear dispersion along the $k_x$ and $k_y$ directions but quadratic dispersion along the $k_z$ direction. Hence, the zero energy solution exists for $(\kappa_{x_\pm}, k_y^0, \pi)$.

2. For $\delta t > \delta E$, there are four values of $\vec{k}$ which yield a zero energy solution, the following $(\kappa_x^\pm, k_{y^0}, \kappa_{z_\pm})$ where $\kappa_z = \cos^{-1}(\frac{\delta E}{2\delta t_z})$ ($\cos(k_z)$ crosses the $\frac{\delta E}{2\delta t_z}$ line twice when $k_z$ varies from 0 to $2\pi$). Expanding $Y$ around $\kappa_z$, we find that $Y(k_z) = 2\delta t_z \sin(\kappa_z) k_z$. Since $\sin(\kappa_z)$ is a constant, the dispersion is linear along $k_z$ as well (it is linear along the $k_x$ and $k_y$ directions before adding the Rashba term which simply shifts them for an appropriate value of the $\lambda$ parameter.). Next, we will analyze how the inclusion of the Hubbard U term changes the Weyl physics.

### C. The effect of the Hubbard U

In order to analyze the role of Coulomb correlations in the Weyl physics, we add a Hubbard U term $U_A$ on the A orbital and a $U_B$ on the B orbital, where $U_x = f_x U, x \in A, B$ such that $f_x$ denotes the percentage of the Mo-$d$ orbital in the x orbital and $f_A \neq f_B$. For the physics we are interested in, using two different Hubbard U terms is qualitatively similar to using only one U term and setting the other to zero. Hence, we will set $U_B = 0$ and write $U_A = g(U)$ where $g(U)$ is some function of U proportional to the percentage of the $d$ orbital. These considerations yield the following Hamiltonian:

$$\hat{H} = \sum_k c_k^\dagger H_{3D}(\mathbf{k}) c_k + g(U) \sum_{i \in A} \hat{n}_{i\uparrow} \hat{n}_{i\downarrow} \tag{19}$$

where, $H_{3D}(\mathbf{k})$ is defined by Eqn. 18 and $c_k\dagger = (c_{k\uparrow}^{A\dagger}, c_{k\uparrow}^{B\dagger}, c_{k\downarrow}^{A\dagger}, c_{k\downarrow}^{B\dagger})$. Writing $\hat{n}_{i\sigma} = \langle n_{i\sigma} \rangle + (\hat{n}_{i\sigma} - \langle n_{i\sigma} \rangle)$, where the second term is the fluctuation about the average term, we obtain the following mean-field Hubbard Hamiltonian:

$$\begin{aligned} \hat{H}_{MF} = \sum_k c_k^\dagger H_{3D}(\mathbf{k}) c_k + g(U) \sum_{i \in A, \sigma} \hat{n}_{i\sigma} \langle n_{i\bar{\sigma}} \rangle \\ + g(U) \sum_{i \in A} \langle \hat{n}_{i\uparrow} \rangle \langle \hat{n}_{i\downarrow} \rangle \hat{I}, \end{aligned} \tag{20}$$

where $\sigma$ and $\bar{\sigma}$ denote spins of opposite flavors.

Since $MoTe_2$ is nonmagnetic, $\langle \hat{n}_{i\uparrow} \rangle = \langle \hat{n}_{i\downarrow} \rangle = \frac{1}{2}$. Then we obtain:

$$\hat{H} = \sum_k c_k^\dagger H_0(k) c_k + \frac{g(U)}{2} \sum_{k,\sigma} \hat{n}_{k\sigma}^A + \frac{g(U)N}{4}, \tag{21}$$

where, $N$ is the total number of lattice sites. Eqn. 21 reduces to a form similar to Eqn. 18 except of the addition of $\frac{g(U)}{4}$ term in the identity and the diagonal term is replaced by $Y = [\delta E - 2\delta t_z \cos(k_z c) + \frac{g(U)}{4}]$. $Y = 0$ as long as $\cos(k_z c) = \frac{(\delta E + \frac{g(U)}{4})}{2\delta t_z}$. Hence, the Weyl point shifts as a function of $U$ and finally gaps out for large enough $U$ such that $|\delta E + \frac{g(U)}{4}| > 2|\delta t_z|$.


[1] P. Giannozzi, S. Baroni, and N. B. et al, J. Phys.: Condens. Matt. **21**, 395502 (2009).
[2] J. P. Perdew, K. Burke, and M. Ernzerhof, Phys. Rev. Lett. **77**, 3865 (1996).
[3] D. R. Hamann, Phys. Rev. B **88**, 085117 (2013).
[4] A. I. Liechtenstein, V. I. Anisimov, and J. Zaanen, Phys. Rev. B **52**, R5467 (1995).
[5] A. Kokalj, J. Mol. Graph. Model. **17**, 176 (1999).
[6] P. Rourke and S. Julian, Comput. Phys. Commun. **183**, 324 (2012).
[7] A. A. Mostofi, J. R. Yates, G. Pizzi, Y.-S. Lee, I. Souza, D. Vanderbilt, and N. Marzari, Comput. Phys. Commun. **185**, 2309 (2014).
[8] Q. Wu, S. Zhang, H.-F. Song, M. Troyer, and A. A. Soluyanov, Comput. Phys. Commun. **224**, 405 (2018).
[9] D. Rhodes, R. Schönemann, N. Aryal, Q. Zhou, Q. R. Zhang, *et al.*, Phys. Rev. B **96**, 165134 (2017).
[10] M. Lindroos, S. Sahrakorpi, and A. Bansil, Phys. Rev. B **65**, 054514 (2002).
[11] J. Pendry, Surf. Sci. **57**, 679 (1976).
[12] C. Caroli, D. Lederer-Rozenblatt, B. Roulet, and D. Saint-James, Phys. Rev. B **8**, 4552 (1973).
[13] Z.-H. Zhu, C. N. Veenstra, G. Levy, A. Ubaldini, P. Syers, N. P. Butch, J. Paglione, M. W. Haverkort, I. S. Elfimov, and A. Damascelli, Phys. Rev. Lett. **110**, 216401 (2013).
[14] A. A. Burkov and L. Balents, Phys. Rev. Lett. **107**, 127205 (2011).
[15] S. Ganeshan and S. Das Sarma, Phys. Rev. B **91**, 125438 (2015).
